# Supplementary material for: Explainable and Transferable Adversarial Attack for ML-Based Network Intrusion Detectors
Source: arXiv:2401.10691 source file (2024-01-19)
Supplement: Supplementary file 1 [file 8-appendix.tex]

\subsection{Feature Additive Importance}
We begin by introducing two notions about the predictive power of feature subsets and the Shaley value of cooperative game theory.

\noindent\textbf{Predictive Power of Feature Subsets.}
As shown in Section~\ref{sec-overview}, considering ML-based NIDSs task where a model $f$ is used to predict the response variable $\mathbf{y}$ given an input $\mathbf{x}$, where $\mathbf{x}$ consists of individual features $(x_1, x_2, . . . , x_n)$.
Our view is that the importance of a feature should correspond to how much predictive power it provides to the model.
To facilitate the evaluation how much $f$'s performance degrades when features are removed, spurred by \cite{covert2020understanding}, we first define the average benefit function for a subset $f_\mathcal{N}$ as $f_{\mathcal{N}}\left(x_{\mathcal{N}}\right)=\mathbb{E}\left[f(\mathbf{x}) \mid \mathbf{x}_{\mathcal{N}}=x_{\mathcal{N}}\right]$.
To define predictive power $v_f$ as a quantity that increases with model accuracy as follows:
\begin{equation}
    v_{f}(\mathcal{N})=\underbrace{\mathbb{E}\left[\ell\left(f_{\varnothing}\left(\mathbf{x}_{\varnothing}\right), \mathbf{y}\right)\right]}_{\text {Mean prediction }}-\underbrace{\mathbb{E}\left[\ell\left(f_{\mathcal{N}}\left(\mathbf{x}_{\mathcal{N}}\right), \mathbf{y}\right)\right]}_{\text {Using features } \mathbf{x}_{\mathcal{N}}}.
\end{equation}

\noindent\textbf{Shapley Value.}
The Shapley value \cite{covert2020understanding} in cooperative game theory is widely regarded as an equitable distribution of the importance or contribution of each player in the game, and it describes the marginal contributions of the coalition faithfully.
Moreover, the Shapley value has been shown to satisfy four desirable properties, i.e., linearity, nullity, symmetry, and efficiency properties. It thus is regarded as a fair way to allocate the total reward to each player.
Specifically, given a multiplayer $N =\{1,2,3,...,n\}$ game, some players cooperate to win the high rewards of the game.
Let $\mathcal{N}\subseteq N$ denote all potential subsets of $N$, and let $\nu (\cdot )$ denote the reward function.
The Shapley value is designed to divide fairly and distribute the total reward to each player.
$\nu (\mathcal{N})$ represents the reward obtained by a set of player $\mathcal{N}\subseteq N$.
The Shapley value $\varphi (i|N)$ unbiasedly measures the contribution of the $i$-th player to the total reward gained by all players in $N$, as follows:
\begin{equation}
    \varphi(i \mid N)=\sum_{\mathcal{N} \subseteq N \backslash\{i\}} \frac{|\mathcal{N}| !(n-|\mathcal{N}|-1) !}{n !}(v(\mathcal{N}\cup\{i\})-v(\mathcal{N})).
\end{equation}

\noindent\textbf{Feature Additive Importance (FAI).}
Using the feature subset predictive power function and the Shapley value, we improve a method for determining the importance of features, called Feature Additive Importance (FAI).
Each Shapley value $\varphi(N)$ is a weighted average of the incremental changes from adding $i$ to subsets $\mathcal{N}\subseteq N \backslash\{i\}$.
Accordingly, FAI value $\varrho (v_f)$ indicates the level of importance of each feature.
And solving the FAI value becomes the following optimization problem, but it is an NP-Hard problem.
\begin{equation}
    \min _{\varrho_{1}, \ldots, \varrho_{d}} \sum_{\mathcal{N} \subseteq N} \frac{n-1}{\left({ }_{|\mathcal{N} |}^{n}\right)|\mathcal{N}|(n-|\mathcal{N}|)}\left(\sum_{i \in \mathcal{N}} \varrho_{i}-v_{f}(\mathcal{N})\right)^{2}
    \end{equation}
We now consider how to calculate FAI values $\varrho_i(x)$ efficiently.
We begin by discarding features with no mutual information.
Moreover, we use random sampling subsets of features $\mathcal{N}\subseteq N$.
Finally, we sample missing features $\mathbf{x}_{\overline{\mathcal{N}}}$ from its marginal distribution, as in \cite{covert2020understanding}.
Our approach for calculating FAI is displayed below in Algorithm~\ref{alg-fai}.
\label{appen-fai}
\begin{algorithm}
    \caption{Approximate Calculation of FAI}
    \label{alg-fai}
    \begin{algorithmic}[1]
        \Require data $ \{ {\mathbf{x}^i,\mathbf{y}^i} \}^\mathcal{I}_{i=1}$, model $f$, loss function $\ell$, outer samples $p$, inner samples $q$. 
        Initialize $\hat{\varrho}_1=0$,$\hat{\varrho}_2=0$,$\ldots$,$\hat{\varrho}_d=0$, $f_{\varnothing}(X_\varnothing)$ = $\frac{1}{\mathcal{I}} \Sigma^\mathcal{I}_{i=1}f(\mathbf{x}_i)$
        \Ensure FAI values $\frac{\hat{\varrho}_i}{p}$
        \If{$I(Y;X^i)<\epsilon $}
        \State $\varrho_i=0$
        \EndIf
        \For{$i=1$ \textbf{to} $p$}
        \State Sample $(x,y)$ from $\{ {x^i,y^i} \}^\mathcal{I}_{i=1}$ 
        \State Sample $\mathcal{P}$, a permutation of $N$
        \State $\mathcal{N}=\varnothing$
        \State $loss_{\_}$= $\ell(f_{\varnothing},y)$
        \For{$j=1$ \textbf{to} $n$}
        \State $\mathcal{N} =\mathcal{N} \cup \{ \mathcal{P}[j]\}$
        \State $y=0$
        \For{$k=1$ \textbf{to} $q$}
        \State Sample $x^k_{\overline{\mathcal{N}}} \sim \varpi(x_{\overline{\mathcal{N}}})$
        \State $y=y+f(x_\mathcal{N},x^k_{\overline{\mathcal{N}}})$
        \EndFor
        \State $\overline{y}=\frac{y}{q}$
        \State $loss$ = $\ell(\overline{y},y)$
        \State $\Delta $ = $loss_{\_}$ $-$ $loss$
        \State $\hat{\varrho}_{\mathcal{P}[j]}=\hat{\varrho}_{\mathcal{P} [j]}+\Delta$
        \State $loss_{\_}$ = $loss$
        \EndFor
        \EndFor
        \State \textbf{return} $\frac{\hat{\varrho}_1}{p},\frac{\hat{\varrho}_2}{p},\ldots,\frac{\hat{\varrho}_d}{p}$
    \end{algorithmic}
    
\end{algorithm}

\subsection{Traffic-space Constraints}
\label{appen-contraints}
Below, we introduce how to remap flow-based and packet-based features to meet the traffic-space constraints.
\vspace{-0.1in}
\subsubsection{Flow-based}
We group flow-based features into the following four groups.
The first category of features is those we can modify independently.
The second group of features is dependent on other features. For example, the mean of packet payloads in the forward direction can be calculated using two other features: the total length of forwarding packets payloads and the total number of forwarding packets.
Third, some features cannot be changed because attackers cannot control them.
There is another type of feature in which their value depends on the actual packets of the flow and cannot be calculated by the value of other features.
We directly modify the features that can be modified independently and calculate the second group of features instantly, without modifying the last two groups of features.
\vspace{-0.1in}
\subsubsection{Packet-based}
The packet-based feature extractor extracts the same set of features from a total of five-time windows.
The relationship between packet-based features is very complex. 
In general, modifying one feature in the same time window can affect other features. 
Moreover, there is also a strong connection between features in different time windows, so it is difficult to satisfy the traffic-space constraints after modifying in feature-space entirely.
We modify the features only in a one-time window and consider feature relationships in the same window, such as their weight and mean.
